# Supplementary material for: Spontaneous Oxygen Vacancy Ionization Enhances Water Oxidation on BiVO$_4$
Source: arXiv:2306.09923 ancillary file (2023-06-16)
Supplement: Supplementary file 1 [file supporting.pdf]

# Supporting Information: Spontaneous oxygen vacancy ionization enhances water oxidation on $BiVO_4$

Nicklas Österbacka,[†] Hassan Ouhbi,[†] Francesco Ambrosio,[‡] and Julia Wiktor[*,†]

†*Department of Physics, Chalmers University of Technology, SE-412 96 Gothenburg, Sweden*

‡*Dipartimento di Chimica e Biologia Adolfo Zambelli, Università di Salerno, Via Giovanni Paolo II, I-84084 Fisciano (SA), Italy*

¶*Dipartimento di Scienze, Università degli Studi della Basilicata, Viale dell'Ateneo Lucano, 10-85100 Potenza, Italy*

E-mail: julia.wiktor@chalmers.se

# 1 Computational details

Total energies were evaluated using the Gaussian and Plane Waves method as implemented in `CP2K`.[S1,S2] Core-valence interactions were described with Goedecker-Teter-Hutter pseudopotentials[S3] and the wave functions were expanded using MOLOPT basis sets[S4] of double-$\zeta$ quality for Bi, V, and O, and of triple-$\zeta$ quality for H, along with an auxiliary plane-wave basis set which was defined up to a cutoff of 600 Ry. A truncated variant of the PBE0 functional was used to describe exchange-correlation energies,[S5,S6] with the exact exchange fraction set to 0.22. The Brillouin zone is sampled at the $\Gamma$ point. This yields a fundamental bandgap in good agreement with experiments after including relevant corrections.[S7] The auxiliary density matrix method was used to speed up calculations.[S8] Geometry optimization was considered converged once all forces were below 10 meV/Å. For vibrational analysis the plane-wave cutoff was increased to 800 Ry and the force cutoff decreased to 1 meV/Å. The formation energy of an oxygen vacancy in charge state $q$ can be expressed as:

$$E^f[\mathrm{O}_{\mathrm{vac}}^q] = E_{\mathrm{tot}}[\mathrm{O}_{\mathrm{vac}}^q] - E_{\mathrm{tot}}[\mathrm{BiVO_4}] - \mu_O + qE_F + E_{\mathrm{corr}}, \tag{1}$$

where $E_{\mathrm{tot}}[\mathrm{O}_{\mathrm{vac}}^q]$ is the energy of the oxygen vacancy, $E_{\mathrm{tot}}[\mathrm{BiVO_4}]$ the energy of the corresponding defect-free supercell, $\mu_\mathrm{O}$ the oxygen chemical potential, and $E_F$ the Fermi level referenced to the valence band maximum (VBM). $E_{\mathrm{corr}}$ corrects for spurious image interactions stemming from the finite system size, and we use the scheme of Freysoldt and Neugebauer.[S9] As this scheme was developed for asymmetric slabs, we use asymmetric slab models for computing defect formation energies. We use a value of 68 for the dielectric constant in the main text,[S10] but recalculate the formation energies with other values in Sec. 2 of the SI. We additionally check the robustness of our conclusions with a symmetric slab model in Sec. 3, as well as a lower fraction of exact exchange in Sec. 4.

# 2 Formation energies with different dielectric constants

The dielectric constant can be chosen in different ways; we have used a value of 68 based on experiments. Fig. S1 shows the oxygen vacancy formation energy calculated with dielectric constants of 40, 68, and 100. As can be seen, the subsurface electron polaron level remains well below the charge transition level (CTL), and the conclusions in the main paper are not sensitive to this choice.

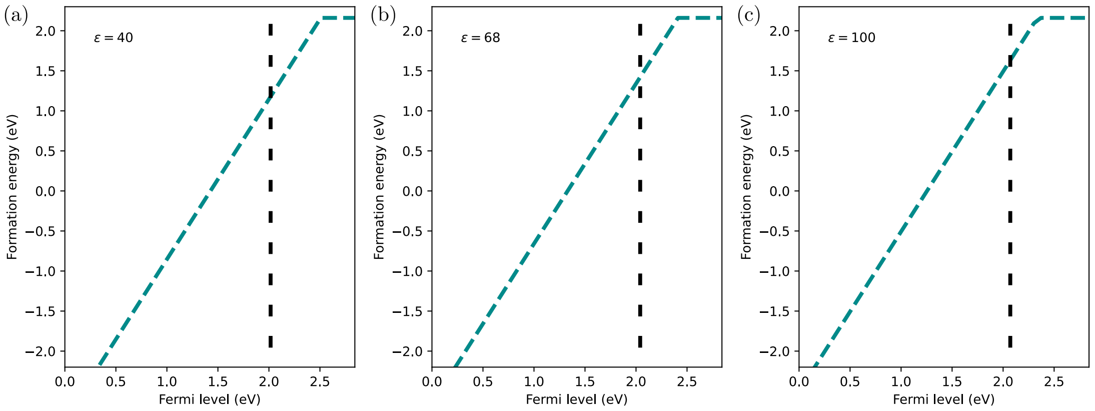


Figure S1: Surface oxygen vacancy formation energies with finite-size corrections calculated with dielectric constants of (a) 40, (b) 68, and (c) 100. The vertical lines represents the charge transition level of the polaron.

# 3 Formation energies with symmetric slabs

As discussed in the main paper, our results contradict those of Wang *et al.*[S11] To ensure that the discrepancy does not arise from methodological differences in the way charged systems are treated, we recalculate the oxygen vacancy formation energies using the correction scheme they propose. It is based on the method of Freysoldt and Neugebauer,[S9] but uses symmetric

slabs instead of asymmetric slabs. The isolated region is taken to be the upper half of the slab, and the final correction is given by the twice the isolated energy minus the periodic energy. We set the dielectric constant to 68.

In the as-published scheme of Freysoldt and Neugebauer, the model charge is placed where it cancels any spurious net dipole across the slab, ensuring a reasonable placement as long as the underlying density functional theory (DFT) model is sound. Any spurious dipole moment is cancelled with a symmetric slab, however, meaning that there is no inherent mechanism for correct charge placement. Instead, we here place the model charges as we did in the asymmetric case in the main paper.

The resulting formation energies are shown in Fig. S2. As clearly shown, the CTL remains above the electron polaron level, and the surface oxygen vacancy is expected to be ionized no matter the Fermi level. The ambiguity in where model charges should be placed makes using this symmetric-slab approach precarious, however.

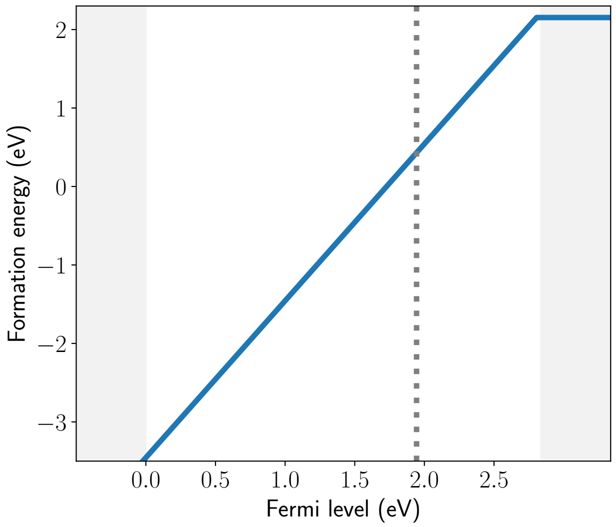


Figure S2: Formation energies for the surface oxygen vacancy, calculated with symmetric slabs. The grey shaded areas represent the band edges and the vertical line represents the charge transition level of the polaron.

# 4 Formation energies with different fraction of exact exchange and PBE+U

A fraction of 22 % exact exchange was used in the main paper, but other values have been used in literature. Based on Koopman's condition, Faletta and Pasquarello found that a value of 14 % was optimal with a plane-wave basis set in Quantum Espresso.[S12] Reoptimizing the defect structures discussed in the main paper with 14 % exact exchange results in the formation energies shown in Fig. S3. Note that the band edge corrections are the same as for the 22 % case. The (0/+2) charge transfer level now lies outside of the bandgap, indicating that the excess electrons stemming from the vacancy are stabler as polarons in locally stoichiometric regions of the material. We note that the band-edge corrections applied here were computed with 22 % exact exchange, which does not affect the separation between the two charge transition levels.

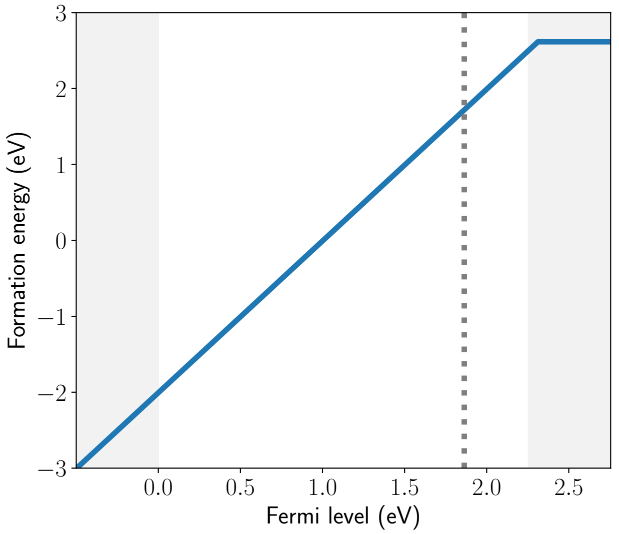


Figure S3: Formation energies for the surface oxygen vacancy calculated with 14 % exact exchange. The grey shaded areas represent the band edges and the vertical line represents the charge transition level of the polaron.

PBE+U is another approach commonly used when modelling defects and polarons in bismuth vanadate. Wang *et al.* used an effective U value of 2.7 eV in their study of the surface oxygen

vacancy in the material. Reoptimizing the defect structures using PBE+U along with this effective U value yields the defect formation energies shown in Fig. S4. No band-edge corrections are applied here. The charge transfer level of the polaron remains below the (+2/0) charge transition level of the oxygen vacancy, and the conclusions of the main paper remain the same even when using PBE+U.

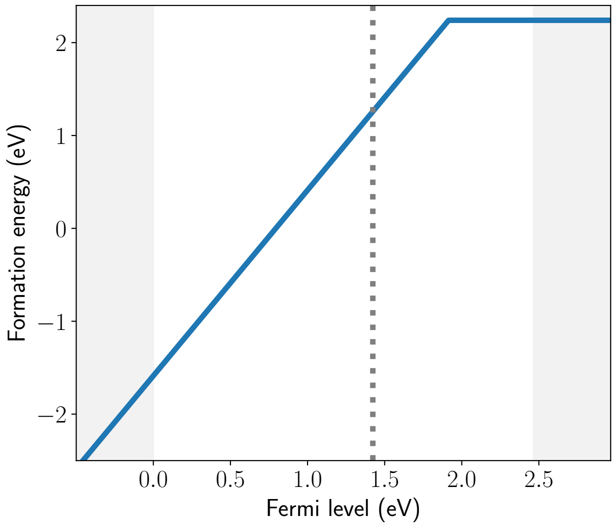


Figure S4: Formation energies for the surface oxygen vacancy calculated with PBE+U and an effective U of 2.7 eV. The grey shaded areas represent the band edges and the vertical line represents the charge transition level of the polaron.

# 5 Vibrational analysis

As is common within the computational hydrogen electrode method, vibrational entropies for Gibbs free energy differences are computed within the harmonic approximation. All degrees of freedom of the adsorbates are assumed to be vibrational, so translational and rotational contributions are neglected. We also assume that the vibrational spectrum of the substrate is mostly unperturbed by the adsorbates and only compute the vibrational frequencies for a handful of atoms near the adsorbate in each intermediate.

For the pristine case, we include the adsorbate atoms, the surface bismuth atom acting as the active site, as well as the oxygen atom involved in dimer formation. For the neutral

vacancy, we include the adsorbate atoms, the surface vanadium atom closest to the vacancy along with its surrounding oxygen atoms, as well as the subsurface corner-sharing vanadium atom along with its oxygen atoms. For the ionized case, we include the adsorbate atoms, the vanadium atom closest to the vacancy along with its three remaining oxygen atoms, the oxygen atom forming the bridge between the surface and subsurface vanadium atoms, as well as the surface oxygen atom onto which a hydrogen is adsorbed for the $*$OOH intermediate. Renders of the adsorbate-free surfaces are shown in Fig. S5, with the atoms not considered in the vibrational analysis transparent.

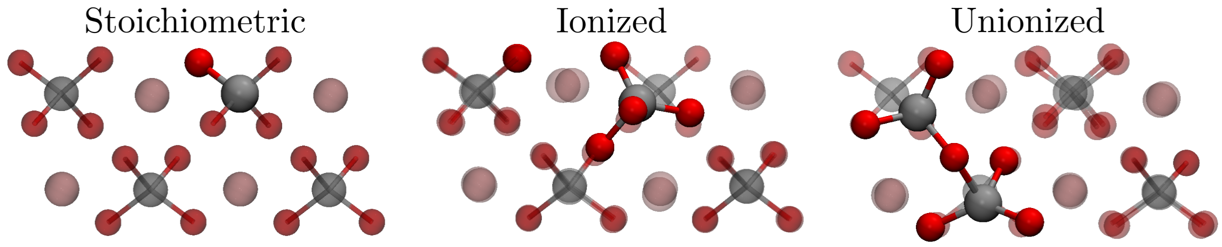


Figure S5: Renders of the two topmost layers of the adsorbate-free slabs considered in this work. The atoms not included in vibrational analysis are transparent.

## References

(S1) Lippert, G.; Hutter, J.; Parrinello, M. A Hybrid Gaussian and Plane Wave Density Functional Scheme. *Mol. Phys.* **1997**, *92*, 477–487.

(S2) Kühne, T. D.; Iannuzzi, M.; Del Ben, M.; Rybkin, V. V.; Seewald, P.; Stein, F.; Laino, T.; Khaliullin, R. Z.; Schütt, O.; Schiffmann, F.; Golze, D.; Wilhelm, J.; Chulkov, S.; Bani-Hashemian, M. H.; Weber, V.; Borštnik, U.; Taillefumier, M.; Jakobovits, A. S.; Lazzaro, A.; Pabst, H.; Müller, T.; Schade, R.; Guidon, M.; Andermatt, S.; Holmberg, N.; Schenter, G. K.; Hehn, A.; Bussy, A.; Belleflamme, F.; Tabacchi, G.; Glöß, A.; Lass, M.; Bethune, I.; Mundy, C. J.; Plessl, C.; Watkins, M.; VandeVondele, J.; Krack, M.; Hutter, J. CP2K: An Electronic Structure and Molecular

Dynamics Software Package - Quickstep: Efficient and Accurate Electronic Structure Calculations. *J. Chem. Phys.* **2020**, *152*, 194103.

(S3) Goedecker, S.; Teter, M.; Hutter, J. Separable Dual-Space Gaussian Pseudopotentials. *Phys. Rev. B* **1996**, *54*, 1703–1710.

(S4) VandeVondele, J.; Hutter, J. Gaussian Basis Sets for Accurate Calculations on Molecular Systems in Gas and Condensed Phases. *J. Chem. Phys.* **2007**, *127*, 114105.

(S5) Perdew, J. P.; Ernzerhof, M.; Burke, K. Rationale for Mixing Exact Exchange with Density Functional Approximations. *J. Chem. Phys.* **1996**, *105*, 9982–9985.

(S6) Guidon, M.; Hutter, J.; VandeVondele, J. Robust Periodic Hartree-Fock Exchange for Large-Scale Simulations Using Gaussian Basis Sets. *J. Chem. Theory Comput.* **2009**, *5*, 3010–3021.

(S7) Wiktor, J.; Reshetnyak, I.; Ambrosio, F.; Pasquarello, A. Comprehensive modeling of the band gap and absorption spectrum of $BiVO_4$. *Phys. Rev. Mater.* **2017**, *1*, 022401.

(S8) Guidon, M.; Hutter, J.; VandeVondele, J. Auxiliary Density Matrix Methods for Hartree-Fock Exchange Calculations. *J. Chem. Theory Comput.* **2010**, *6*, 2348–2364.

(S9) Freysoldt, C.; Neugebauer, J. First-Principles Calculations for Charged Defects at Surfaces, Interfaces, and Two-Dimensional Materials in the Presence of Electric Fields. *Phys. Rev. B* **2018**, *97*, 205425.

(S10) Wee, S.-H.; Kim, D.-W.; Yoo, S.-I. Microwave Dielectric Properties of Low-Fired $ZnNb_2O_6$ Ceramics with $BiVO_4$ Addition. *Journal of the American Ceramic Society* **2004**, *87*, 871–874.

(S11) Wang, W.; Strohbeen, P. J.; Lee, D.; Zhou, C.; Kawasaki, J. K.; Choi, K.-S.; Liu, M.; Galli, G. The Role of Surface Oxygen Vacancies in $BiVO_4$. *Chem. Mater.* **2020**, *32*, 2899–2909.

(S12) Falletta, S.; Pasquarello, A. Polarons Free from Many-Body Self-Interaction in Density Functional Theory. *Phys. Rev. B* **2022**, *106*, 125119.
